# Supplementary material for: Robust Infidelity: When Faithfulness Measures on Masked Language Models Are Misleading
Source: arXiv:2308.06795 source file (2024-05-31)
Supplement: Supplementary file 1 [file 99-appendix.tex]

%\section{Additional Results}
